# Supplementary material for: Match me if you can: Semi-Supervised Semantic Correspondence Learning with Unpaired Images
Source: arXiv:2311.18540 source file (2024-10-11)

Clean

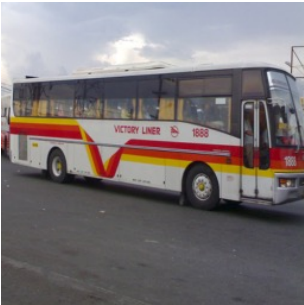

Gaussian Noise

Severity = 1

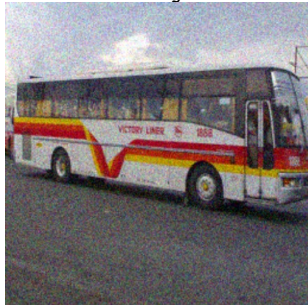

Severity = 2

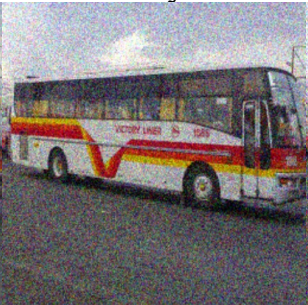

Severity = 3

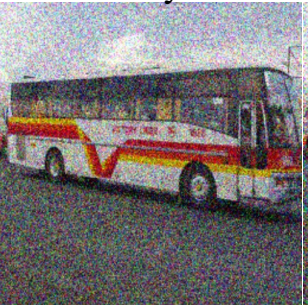

Severity = 4

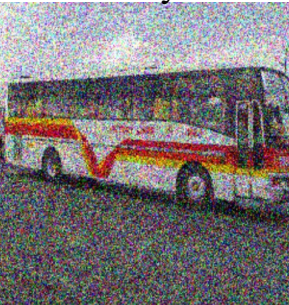

Severity = 5

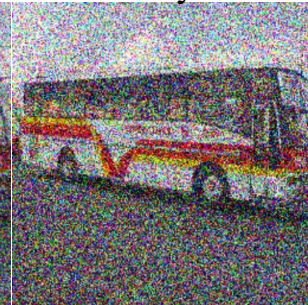

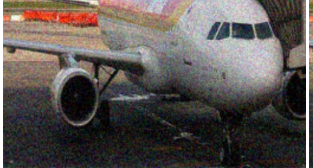

Frost

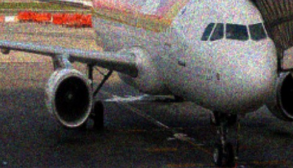

Fog

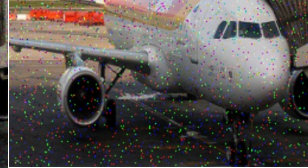

Brightness

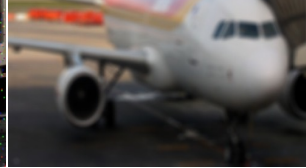

Contrast

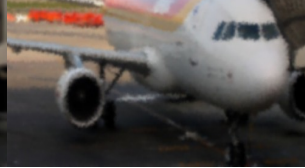

Elastic

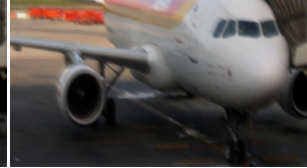

Pixelate

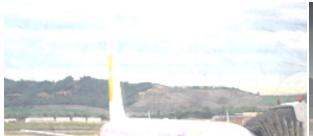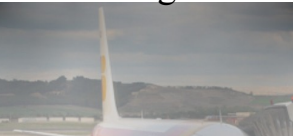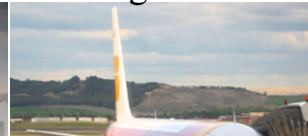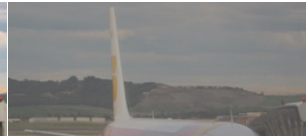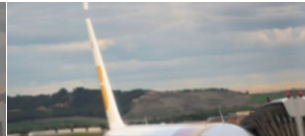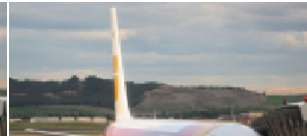

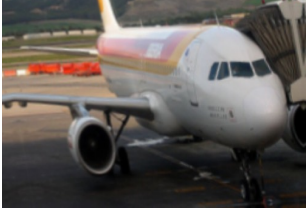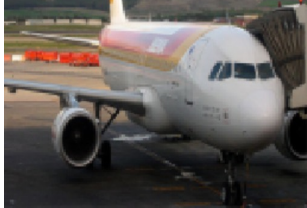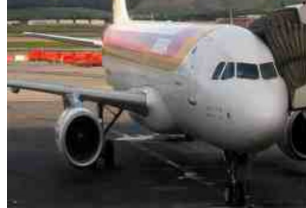

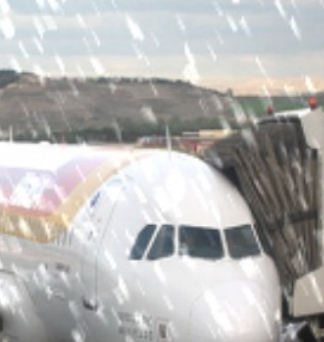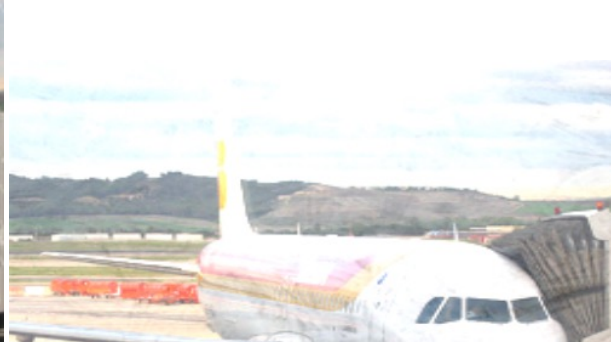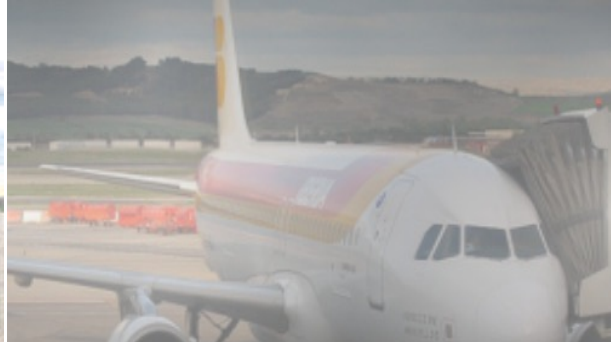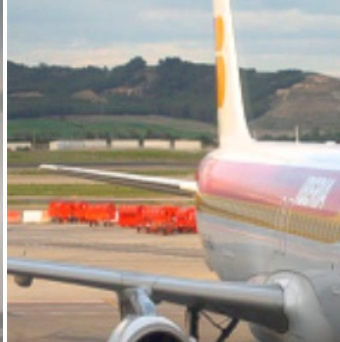

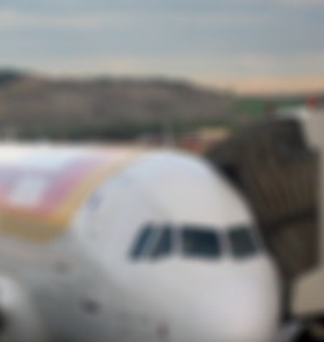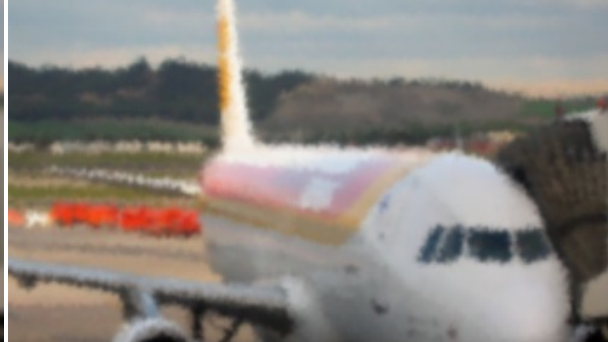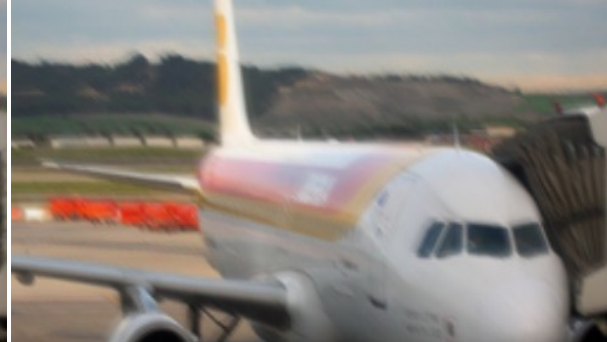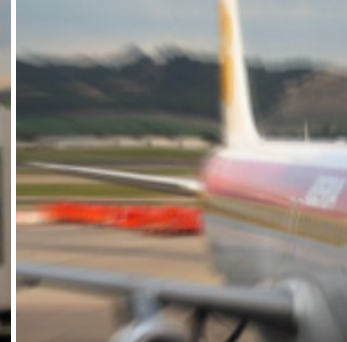

Supplement: Supplementary file 1 [file rob_all_1.pdf]
